# Supplementary material for: Machine learning exploration of binding energy distributions of H2O at astrochemically relevant dust grain surfaces
Source: arXiv:2602.11050 ancillary file (2026-02-11)
Supplement: Supplementary file 1 [file binding_energy_paper_arxiv_SI.pdf]

# Supporting Information: Machine learning exploration of binding energy distributions of $H_2O$ at astrochemically relevant dust grain surfaces

Anant Vaishnav, Niels M. Mikkelsen, and Mie Andersen*

*Center for Interstellar Catalysis, Department of Physics and Astronomy, Aarhus University, Aarhus C 8000, Denmark*

E-mail: mie@phys.au.dk

Table S1: Benchmarking for $H_2O$ on graphene

| Model / functional | Adsorption energy (meV)* |
|---|---|
| PBE-D4 (this work) | −97 |
| PaiNN model (this work) | −77 |
| DMC[S1] | −90 |
| PBE-D4[S1] | −104 |
| PBE0-D4[S1] | −103 |

**Without zero-point vibrational energy corrections. The structure used to evaluate the adsorption energy is 0-leg $H_2O$ on graphene as described in Ref. S1.*

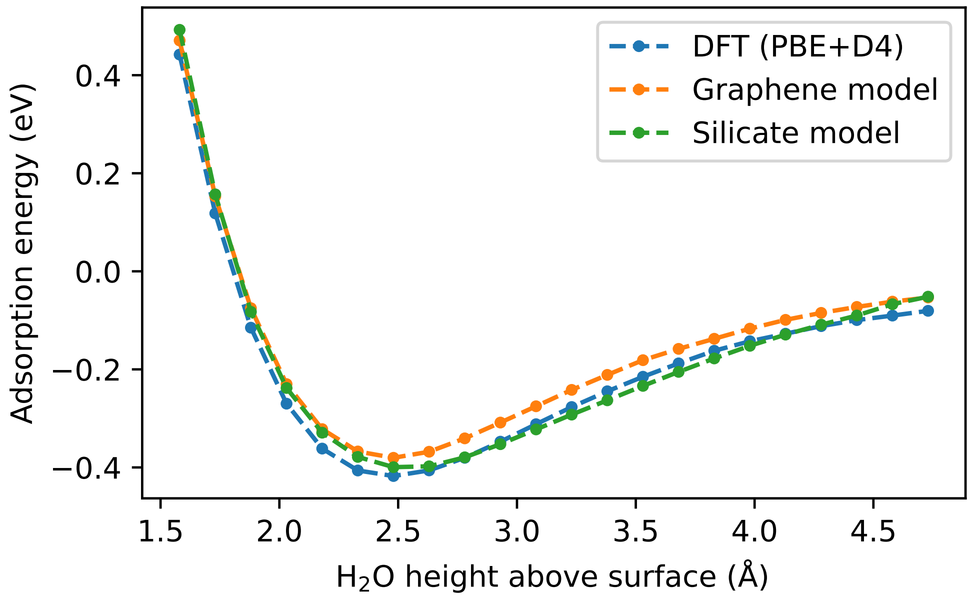


Figure S1: Comparison of energy predictions between DFT with D4 dispersion corrections and the graphene and silicate PaiNN models. The adsorption energy is for a $H_2O$ adsorbate on an amorphous $H_2O$ surface.

Table S2: Benchmarking for $H_2O$ on the (010) facet of forsterite

| Model / functional | Adsorption energy (eV)* |
|---|---|
| PBE-D3 (this work) | −1.33 |
| PaiNN model (this work) | −1.14 |
| B3LYP-D2[S2] | −1.17 |

**Without zero-point vibrational energy corrections. The structure used to evaluate the adsorption energy is similar to Figure 5(a) in Ref. S2, where the $H_2O$ has one hydrogen bond with a surface O.*

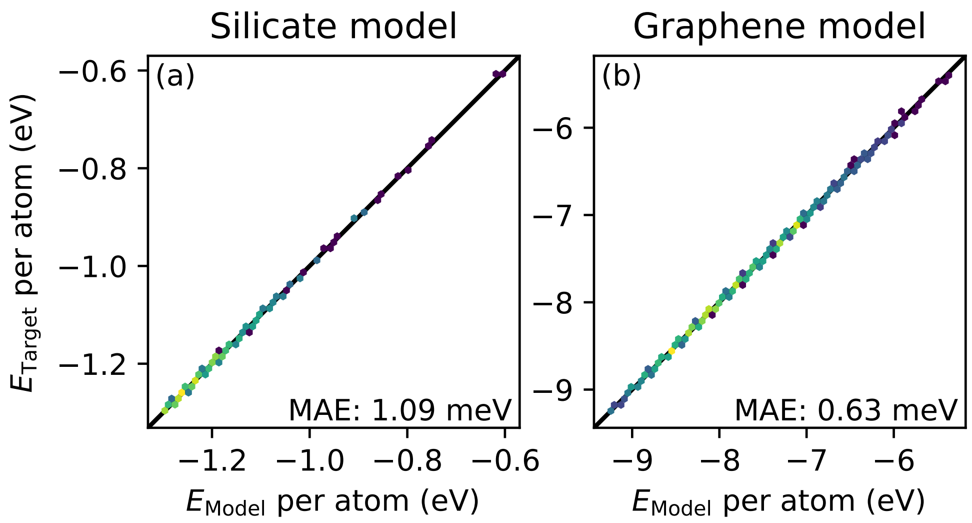


Figure S2: Parity plots of energy per atom in the test sets for the silicate and graphene PaiNN models. The color of the hexagons represent the density of data points from low density (dark blue) to high density (yellow).

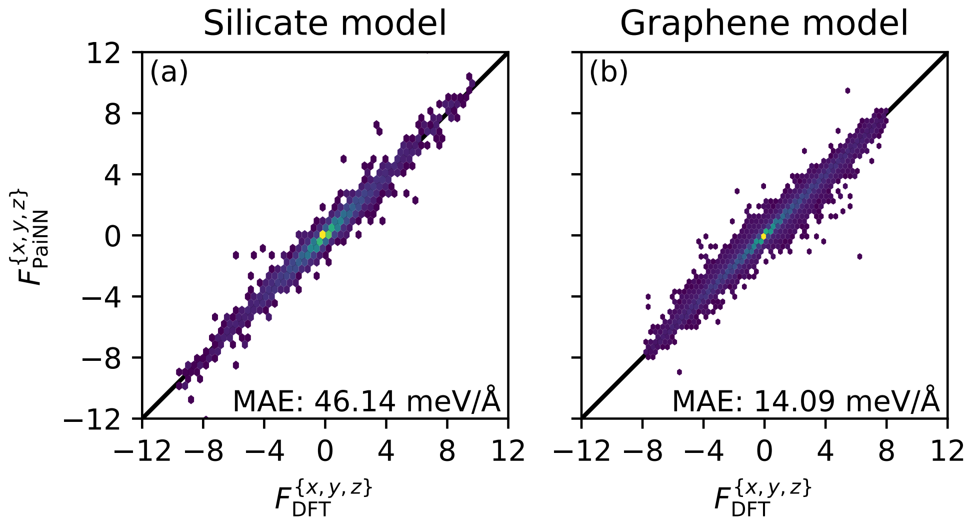


Figure S3: Parity plots of force components in the test sets for the silicate and graphene PaiNN models. The color coding is as in Figure S2.

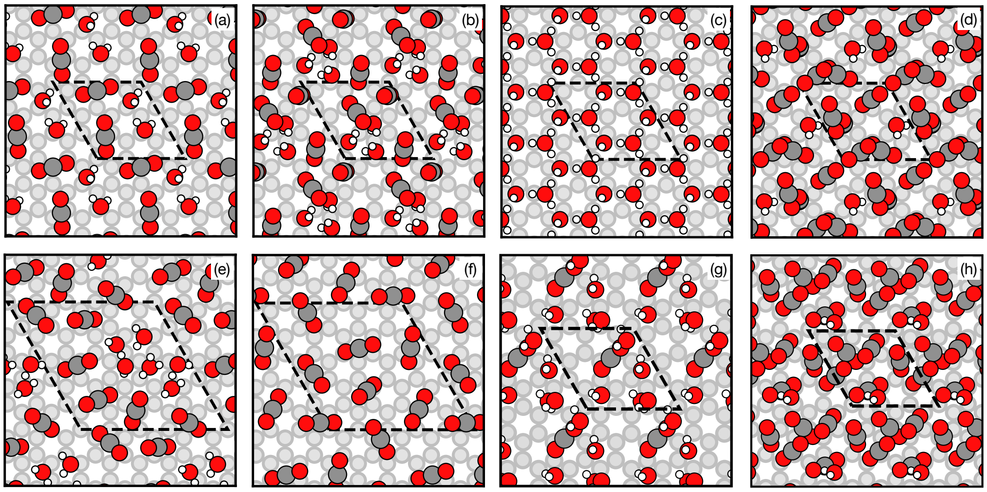


Figure S4: Examples of structures in the data set for the graphene model. (a-d): Structures from structure searches using GOFEE with a $3 \times 3$ graphene cell. (e-f): Structures from structure searches using a $5 \times 5$ cell. (g-h): Structures from AIMD at different mixing ratio of $H_2O$ and $CO_2$.

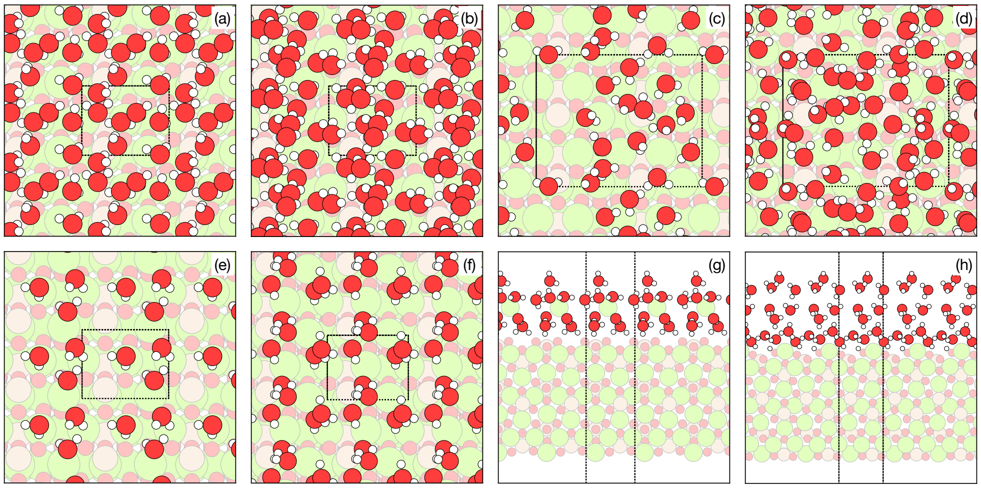


Figure S5: Examples of structures in the data set for the silicate model. (a) and (b) show structures from GO searches in the small cell, (c) and (d) from GO searches in the large cell and (e) and (f) from AIMD with different number of water molecules. (g) is the side view of a structure showing Mg extraction encountered during long MD runs with the initial model. (h) is the side view of a structure showing water dissociation near the surface encountered during 500 K MD runs with the initial model. Structures similar to (g) and (h) were DFT evaluated and added to the data set to rectify the unphysical behavior of the initial model.

# References

(S1) Brandenburg, J. G.; Zen, A.; Alfè, D.; Michaelides, A. Interaction between water and carbon nanostructures: How good are current density functional approximations? *The Journal of Chemical Physics* **2019**, *151*, 164702.

(S2) Molpeceres, G.; Rimola, A.; Ceccarelli, C.; Kästner, J.; Ugliengo, P.; Maté, B. Silicate-mediated interstellar water formation: a theoretical study. *Monthly Notices of the Royal Astronomical Society* **2018**, *482*, 5389–5400.
